# Supplementary material for: Extreme Point Supervised Instance Segmentation
Source: arXiv:2405.20729 source file (2024-06-04)
Supplement: Supplementary file 1 [file tab_sup_mil_weight.tex]

% Please add the following required packages to your document preamble:
% \usepackage{graphicx}
\begin{table}[ht]
\centering
\resizebox{0.5\linewidth}{!}{% Adjust the 0.8 to whatever suits your needs
\begin{tabular}{cccc}
\toprule
$\lambda_{mil}$ & AP & AP_{50} & AP_{75} \\
\midrule
2        & 39.7 & 67 & 40.1      \\ 
\rowcolor[HTML]{EFEFEF}10        & \textbf{40.4} & \textbf{67.4} & \textbf{41.4}      \\ 
20          & 39.8 & 66.7 & 40.4      \\ 
40          & 39.4 & 66.6 & 39.5      \\  \bottomrule
\end{tabular}%
}
\vspace{-2mm}
\caption{Effect of $\lambda_{mil}$ for the case of  $ | \hat{\mathcal{P}}_\text{FG} \cup \hat{\mathcal{P}}_\text{BG} | = 0 $.}
\label{tab:sup_mil_weight}
\vspace{-4mm}
\end{table}
