# Supplementary material for: Extreme Point Supervised Instance Segmentation
Source: arXiv:2405.20729 source file (2024-06-04)
Supplement: Supplementary file 2 [file tab_sup_point_and_crf_weight.tex]

\begin{table}[ht]
\centering
\begin{minipage}[b]{0.45\linewidth} % Adjust the minipage width as needed
\centering
\resizebox{\linewidth}{!}{%
\begin{tabular}{cccc}
\toprule
$\lambda_{point}$ & AP & AP_{50} & AP_{75} \\
\midrule
0.1        & 40.1 & 66.6 & 41.3      \\ 
\rowcolor[HTML]{EFEFEF}0.5        & \textbf{40.4} & \textbf{67.4} & \textbf{41.4}      \\ 
1          & 38.8 & 65.9 & 39.3      \\ 
2          & 38   & 66.2  & 38.1    \\ 
\bottomrule
\end{tabular}%
}
\caption{Effect of loss coefficient $\lambda_{point}$.}
\label{tab:sup_point_weight}
\end{minipage}
\hfill
\begin{minipage}[b]{0.425\linewidth} % Adjust the minipage width as needed
\centering
\resizebox{\linewidth}{!}{%
\begin{tabular}{cccc}
\toprule
$\lambda_{crf}$ & AP & AP_{50} & AP_{75} \\
\midrule
0.1        & 37.9 & 65.9 & 37.6      \\ 
0.25        & 38.7 & 66.1 & 38.6      \\ 
\rowcolor[HTML]{EFEFEF}0.5          & \textbf{40.4} & \textbf{67.4} & \textbf{41.4}      \\ 
1          & 4   & 66.6  & 40.7    \\ 
\bottomrule
\end{tabular}%
}
\caption{Effect of loss coefficient $\lambda_{crf}$.}
\label{tab:sup_crf_weight}
\end{minipage}
\end{table}
