# Supplementary material for: Extreme Point Supervised Instance Segmentation
Source: arXiv:2405.20729 source file (2024-06-04)
Supplement: Supplementary file 3 [file tab_sup_tau.tex]

\begin{table}[ht]
\centering
\begin{minipage}[b]{0.45\linewidth} % Adjust the minipage width as needed
\centering
\resizebox{\linewidth}{!}{%
\begin{tabular}{cccc}
\toprule
$\tau_{\text{FG}}$ & AP & AP_{50} & AP_{75} \\
\midrule
0.00075        & 38.1 & 65.7 & 38.1      \\ 
\rowcolor[HTML]{EFEFEF}0.001        & 40.4 & 67.4 & 41.4      \\ 
0.00125          & 40.1   & 66.6  & 41.3    \\ 
0.0015          & \textbf{41.1} & \textbf{67.6} & \textbf{42.6}      \\ 
0.002          & 40.9   & 67.6  & 42.4    \\ 
\bottomrule
\end{tabular}%
}
\caption{Effect of $\tau_{\text{FG}}$}
\label{tab:sup_tau_fg}
\end{minipage}
\hfill
\begin{minipage}[b]{0.475\linewidth} % Adjust the minipage width as needed
\centering
\resizebox{\linewidth}{!}{%
\begin{tabular}{cccc}
\toprule
$\tau_{\text{BG}}$& AP & AP_{50} & AP_{75} \\
\midrule
-0.00005        & 39.7 & 66.6 & 40.7      \\ 
\rowcolor[HTML]{EFEFEF}-0.0001        & \textbf{40.4} & \textbf{67.4} & \textbf{41.4}      \\ 
-0.00015         & 39.6 & 66.2 & 40.3      \\ 
-0.0002           & 38.8 & 65.9 & 39.1      \\ 
\bottomrule
\end{tabular}%
}
\caption{Effect of $\tau_{\text{BG}}$}
\label{tab:sup_tau_bg}
\end{minipage}
\end{table}
